# Supplementary material for: Automated Detection of Short-term Slow Slip Events in Southwest Japan
Source: arXiv:2202.12414 source file (2025-09-20)
Supplement: Supplementary file 1 [file supplement.pdf]

# Detecting change-points in noisy GPS time series with continuous piecewise structures: Supplement

Yiming Ma

*Department of Mathematics and Statistics, University of Otago, Dunedin 9016, New Zealand.*

E-mail: maym@maths.otago.ac.nz

Andreas Anastasiou

*Department of Mathematics and Statistics, University of Cyprus, Nicosia 1678, Cyprus.*

Ting Wang & Fabien Montiel

*Department of Mathematics and Statistics, University of Otago, Dunedin 9016, New Zealand.*

## 1. SSEs simulation

We consider a simplified Cascadia-like model, which consists of a planar frictional interface simulating the thrust fault between a subducting oceanic plate and an overlying continental plate in an elastic half-space, as shown in Fig. S1. It is composed of a seismogenic zone where megathrust earthquakes spontaneously arise, a transition zone where SSEs spontaneously arise, a creeping zone where instabilities cannot spontaneously arise, and an infinitely long zone which is enforced to slide at a constant speed (i.e. the plate velocity  $v_{pl}$ ). We use the following dimensionless system of ODEs to simulate the slip velocity history for the  $i$ -th subfault,

$$\begin{cases} \frac{dv_i}{dt} = \frac{v_i}{a\sigma_i + v_i} \left[ \sum_{j=1}^N K_{ij}(1 - v_j) - \frac{b\sigma_i}{\theta_i}(1 - \theta_i v_j) \right] \\ \frac{d\theta_i}{dt} = 1 - \theta_i v_j, \end{cases} \quad (1)$$

where indices  $i$  and  $j$  refer to different subfaults;  $N$  is the number of the subfaults in our model;  $K_{ij}$  is the kernel coefficient, which quantifies the interactions between the  $i$ -th

and  $j$ -th subfault;  $v_i$  and  $\theta_i$  are the slip rate and a state variable for the  $i$ -th subfault, respectively;  $a$  and  $b$  are experimentally determined constitutive constants. This system is solved by using the adaptive fourth order Runge-kutta method (see more details in Rubin (2008)). Except for the SSE data shown in the main context, we simulate more SSE data with different number of SSEs in a one-year period, shown in Fig. S2.

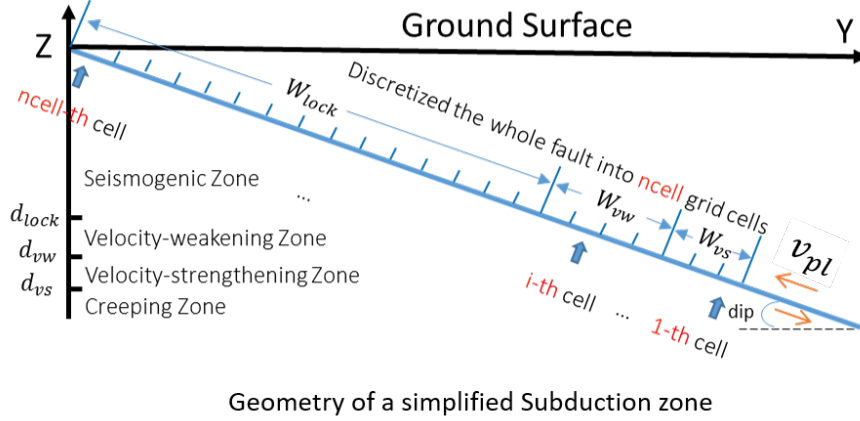

**Fig. S1.** Geometry of a 2D simplified subduction fault, which is composed of a seismogenic zone, a transition zone (velocity-weakening, where SSEs should occur), a creeping zone (velocity-strengthening) and an infinitely long zone forced to slide at the constant velocity of  $v_{plate}$ .

## 2. Additional observations in tests of §2.2

When defining a successful detection in §2.2, the threshold  $v$  should be designated by the users according to their own fields. Fig. S3 shows the dependence of  $R_{sd}$  on different  $v$ . We will obtain a higher  $R_{sd}$  if adapting a larger  $v$ . To investigate the effect of noise levels on the detection accuracy of Isolate-Detect (ID) (Anastasiou and Fryzlewicz, 2021), we plot the quartile distributions of RMSE for each noise level in Fig. S3(b). We first identify the successful detections among the corresponding 10,000 tests for each noise level in the tests shown in Fig. 3(b) of the main context, and then calculate the RMSE for each detection. The quartile values are picked from these calculated RMSE.

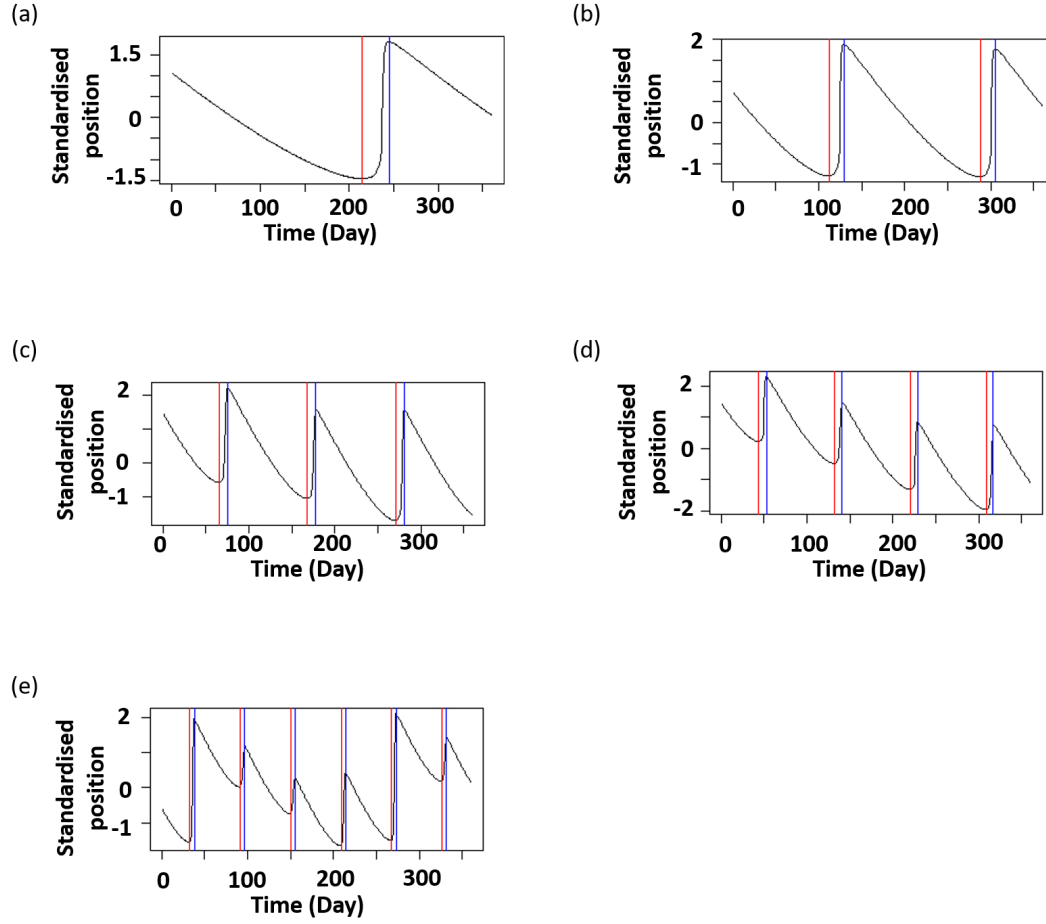

**Fig. S2.** Simulated pure SSE data with different numbers of SSEs in a one-year period: (a) 1; (b) 2; (c) 3; (d) 4; (e) 6. Red vertical lines: the start time of an SSE; blue vertical line: the end time of an SSE.

### 3. Determine the final output of change-points

We verify the validity of taking the mode of each column in  $D$  shown in Eq. (6) to estimate the locations of underlying change-points in noisy data sequences. We first recall tests for a suitable noise level (i.e.  $C_{wn} = 35\%$ ) shown in Fig. 3 (b) as an example. It is sensible that the mode of the number of detected change-points is equal to the number of true change-points (i.e. 10). Among these 10,000 tests, we identify the ones with  $\hat{N} = 10$ , and store the locations of their detected change-points to form the matrix  $D$  shown in Eq. (6). The final output of estimated change-points for this noise

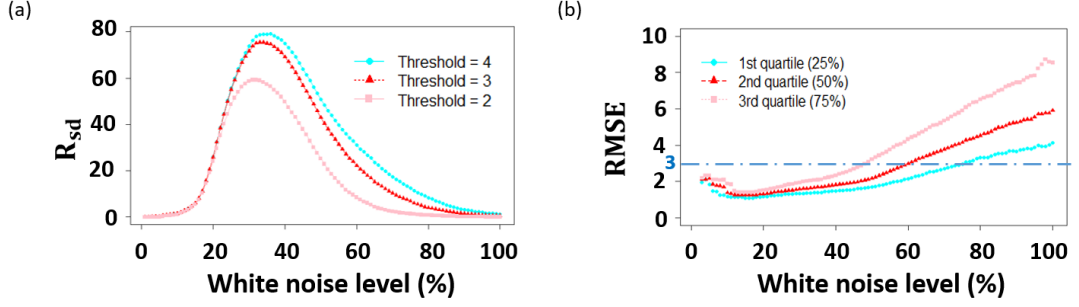

**Fig. S3.** (a) The successful detection percentage  $R_{sd}$  as a function of noise levels against different threshold  $v$ ; (b) The quartile distributions of RMSE as a function of noise levels for ID. The dotted horizontal blue line indicates the threshold that we use in our following tests.

level is (20, 26, 94, 99, 165, 173, 239, 246, 316, 321), which is consistent with the locations of true change-points (i.e. 19, 26, 93, 100, 166, 173, 240, 246, 313, 320). The histogram for each estimated change-point is shown in Fig. S4. The current result confirms that the mode is suitable to estimate the location of true change-points.

#### 4. SSAID performance on more simulated SSE data

We further demonstrate the performance of our method based on the same tests shown in Fig. 6(a) in the main context, but using different underlying SSE signal  $f_t$ . The results are shown in Fig. S5, which are consistent with the observations in the main text (see §4.1.1).

#### 5. Tests on other synthetic signals with piecewise structures

We first verify the general applicability of SSAID to detect change-points in other types of piecewise-non-linear data sequences using simulated signals with known structures. We consider signals with the following structures: (1) piecewise-quadratic; (2) piecewise-exponential; and (3) sinusoidal (see Fig. S6 (a), (c) and (e), respectively). We have  $100 \times 101$  noisy data sequences for each scenario. Fig. S6 (b) and (f) show that for the piecewise-quadratic and the sinusoidal signals, SSAID consistently detects the true change-points successfully when  $C_{wn}$  is sufficiently small (approximately  $\leq 20\%$  for

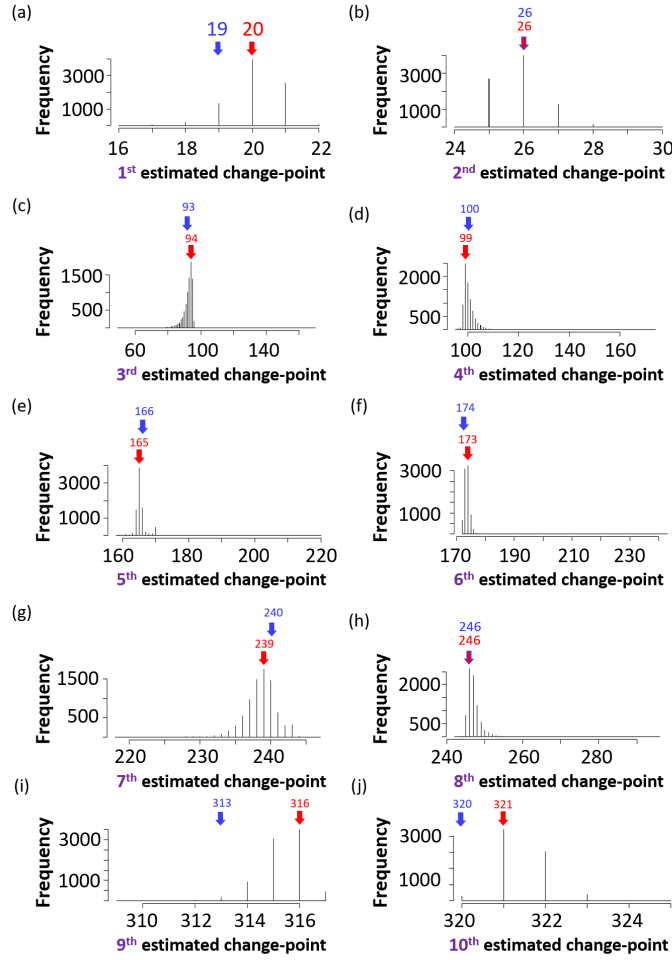

**Fig. S4.** The histogram of different estimated change-points: (a) 1<sup>st</sup>; (b) 2<sup>nd</sup>; (c) 3<sup>rd</sup>; (d) 4<sup>th</sup>; (e) 5<sup>th</sup>; (f) 6<sup>th</sup>; (g) 7<sup>th</sup>; (h) 8<sup>th</sup>; (i) 9<sup>th</sup>; (j) 10<sup>th</sup>. Blue arrows: the locations of true change-points; red arrows: the locations of estimated change-points. The blue-red arrow indicates the estimated change-point is the same as the true one.

piecewise-quadratic;  $\leq 40\%$  for sinusoidal function). SSAID can guarantee successful detection of true change-points, while the successful detection percentage monotonically decreases with  $C_{wn}$ . Our approach performs even better for the piecewise-exponential signal (see Fig. S6 (d)). It finds the correct number of change-points even when  $C_{wn}$  is close to 100%. We also check its adaptability to piecewise-linear signals, and further compare its performance with that of ID. Fig. S6 (h) illustrates SSAID can accurately

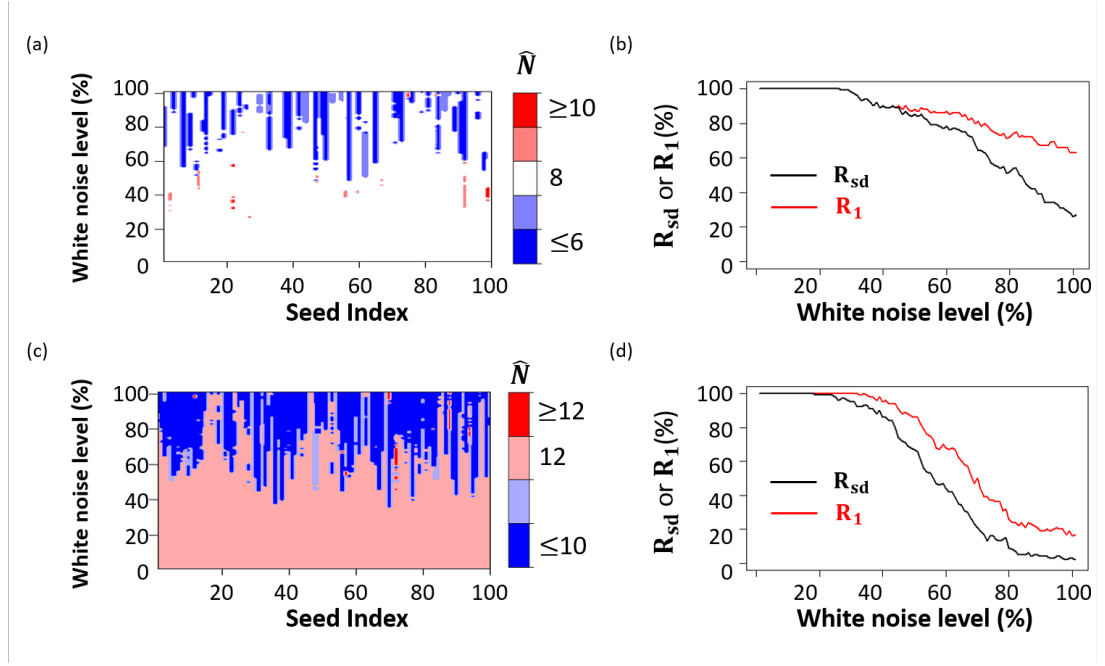

**Fig. S5.** (a) The number of estimated change-points  $\hat{N}$  in each simulated noisy data by our approach; (b) The percentage  $R_1$  (see Eq. (8) in the main context) and  $R_{sd}$  (successful detection percentage) for each white noise level  $C_{wn}$ , out of 100 seeds. The underlying signals  $f_t$  for tests in (a) and (b) are shown in Fig. S2(c) and S2(e), respectively. Their associated numbers of true change-points are 8 and 12, respectively. When calculating the percentage of successful detections  $R_{sd}$ , the threshold  $v = 4$ .

detect true change-points, and improve the  $R_{sd}$  of ID for  $C_{wn} \geq 60\%$ . These four cases indicate that our approach can be applied to a wide variety of signals.

## 6. The pseudocode for SSAID

---

### Algorithm 1: The pseudocode of SSAID

---

**Result:** Estimated change-points for the input data  $X_t$

---

- 1 **Step 1** (Decomposition process): Obtain denoised data with different noise levels  $Y_t^k$  ( $k = 1, \dots, M$ );
  - 2  $R_t^j \leftarrow$  The  $j$ -th decomposed component of  $X_t$  by SSA;
  - 3  $Y_t^k \leftarrow \sum_{j=1}^k R_t^j$ ;
  - 4 **Step 2** (Adding noise in the way of the  $R_{sd}$  improvement scheme): Generate a range of new noisy data  $Z_t^{k,s,m}$  ( $k = 1, \dots, M; s = 1, \dots, L; m = 1, \dots, Q$ ) to guarantee the existence of in-SNL data;
  - 5  $Z_t^{k,s,m} \leftarrow Y_t^k + a_s \omega_t^m$ ;
-

---

```

6 Step 3 (The main part): Identifying in-SNL data among all the  $Z_t^{k,s,m}$ 
   group-by-group, through three condition: (1)  $\hat{H} \neq 0$ ; (2)  $R_2 \geq 50\%$ ; (3)  $\Omega_3 \leq v$ ;
7 for  $k=1:M$  do
8   for  $s=1:L$  do
9     Determine  $\hat{N}^{k,s}$  for the group of  $\mathbf{G}^{k,s} = \{Z_t^{k,s,1}, \dots, Z_t^{k,s,Q}\}$ ;
10    for  $m=1:Q$  do
11       $\hat{N}^{k,s,m} \leftarrow$  The number of estimated change-points for  $Z_t^{k,s,m}$  by ID;
12    end
13     $\hat{H}^{k,s} \leftarrow Mo\{\hat{N}^{k,s,1}, \dots, \hat{N}^{k,s,Q}\}$ ;
14    Condition 1:
15    if  $\hat{H}^{k,s}=0$  then
16      All the members in  $\mathbf{G}^{k,s}$  are marked as ‘NOT in-SNL data’;
17    else
18       $\kappa \leftarrow$  The frequency of the mode  $\hat{H}^{k,s}$  amongst  $\{\hat{N}^{k,s,1}, \dots, \hat{N}^{k,s,Q}\}$ ;
19       $R_2^{k,s} \leftarrow \kappa/Q$ ;
20      Condition 2:
21      if  $R_2^{k,s} < 0.5$  then
22        All the members in the current group  $\mathbf{G}^{k,s}$  are marked as ‘NOT
          in-SNL data’;
23      else
24         $D \leftarrow$  Generate a matrix shown in Eq. (6) which has a size of
           $(\kappa, \hat{H}^{k,s})$ ;
25         $U^{k,s} \leftarrow$  The mode of each column in  $D$ ;
26        Condition 3:
27         $\Omega_3 \leftarrow$  The third quartile (75%) of the RMSE for each group by
          assuming  $U^{k,s}$  as the real change-points for  $Z_t^{k,s}$ ;
28        if  $\Omega_3 > v$  then
29          All the members in the current group  $\mathbf{G}^{k,s}$  are marked as ‘NOT
            in-SNL data’;
30        end
31      end
32    end
33  end
34  Output the number of change-points for  $Y_t^k$ :  $\hat{H}^k \leftarrow Mo\{\hat{H}^{k,1}, \dots, \hat{H}^{k,L}\}$ ;
35 end

```

---

- 
- 
- 36  $\hat{N} \leftarrow Mo\{\hat{H}^1, \dots, \hat{H}^M\}$ , to determine the number of change-points  $\hat{N}$  for  $X_t$ ;
  - 37 Collect all the groups which are not marked as ‘**NOT in-SNL data**’;
  - 38 **Step 4:** Output the final estimated locations of change-points for  $X_t$ ;
  - 39 Pick up all the members with  $\hat{N}^{k,s,m} = \hat{N}$  from in-SNL data, and then store their detected change-points into a new matrix  $D_f$ , which is the same as  $D$  in Eq. (6), but with a different size;
  - 40  $U \leftarrow$  The mode of each column in  $D_f$  is used to estimate the location of change-points in  $X_t$ .
- 

## 7. Determining SNL range for simulated SSE data

We explore the SNL range for the two simulated SSE data in Section 5.3 in the main context (see Fig. 9 (a)). The results show that no SNL can be found for the first SSE data, while the SNL range for the second SSE data is 32 – 121%. We further explore the SNL range for each subset (see different colors in Fig. 9 (a)). The SNLs for the green and red subsets have no common values. This explains why no SNL exists for the first SSE data. The SNLs for the golden and cyan subsets partially overlap in the noise levels 32 – 152%, explaining why we could find the SNLs for the second SSE data.

## 8. Applications to other real data sets

We now apply SSAID to detect change-points in other real-world data sets with piecewise-non-linear structures.

### 8.1. COVID-19 daily new confirmed cases in the US

The first case study here is to look for change-points in COVID-19 daily new confirmed cases in the US. We perform the Anscombe transform on the original data, to make its distribution more consistent with the assumption of Gaussianity for the noise (Anscombe, 1948). Fig. S7 (a) shows that the detected change-points by SSAID with and without a sliding window mostly overlap, except two change-points indicated by the shaded green areas. Most of these detected change-points are consistent with the visual inspection on the trend change of the data itself.

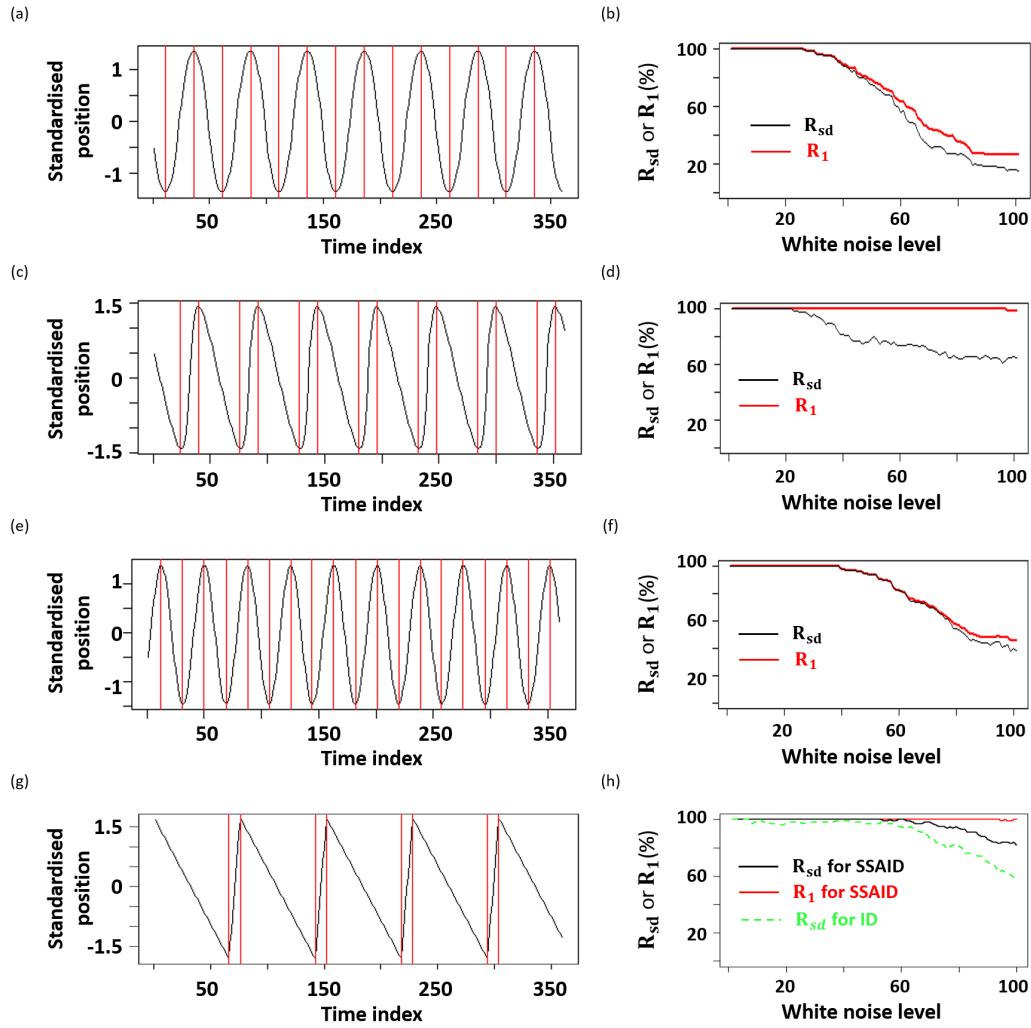

**Fig. S6.** Simulated pure signals with different structures: (a) piecewise-quadratic signal; (c) piecewise-exponential signal; (e) sinusoidal function; (g) piecewise-linear signal. Their corresponding successful detection ratio  $R_{sd}$  and the percentage  $R_1$  (see the definition in §??) are shown in panels (b), (d), (f) and (h), respectively. Red vertical lines: true-change points, defined as the local extrema of the pure signals. The error threshold is 3 when calculating  $R_{sd}$ .

We further elaborate possible reasons that could explain the detected change-points, which can often be associated with the issued dates of government interventions (e.g. lockdown, mass testing or lifting restrictions). Detecting these change-points can further help monitor COVID-19 phase changes, e.g. in terms of its growth rate, which can assist the government assess the effectiveness of their policies on the evolution of the

pandemic (Jiang et al., 2020; Pei et al., 2020). The interventions described in the following context mainly come from the timeline of the COVID-19 pandemic in the United States (2020) in Wikipedia (see [https://en.wikipedia.org/wiki/Timeline\\_of\\_the\\_COVID-19\\_pandemic\\_in\\_the\\_United\\_States\\_\(2020\)#cite\\_note-121](https://en.wikipedia.org/wiki/Timeline_of_the_COVID-19_pandemic_in_the_United_States_(2020)#cite_note-121)) and the report from Schuchat et al. (2020). The first change-point is detected on 9 March 2020, which might result from the order issued by the CDC (Centers for Disease Control and Prevention) on 5 March. This order lifted the restrictions for a coronavirus test so that anyone in the US was allowed to get an COVID-19 test, resulting in a rapid increase. This change-point is also consistent with the syndromic surveillance in counties affected early by the COVID-19 in the US, which did not show an increase in visits for COVID-19-like illness (e.g. fever, cough) until 28 February 2020. We find the second change-point on 02 April 2020, which coincides with the emergent orders from New York state government (i.e. the leading confirmed cases in the US at that time. The New York state government closed all nonessential construction sites on 28 March 2020, and the U.S. Navy medical ship arrived in the New York city to assist with non-COVID operations, relieving land hospitals to stop the city’s growing COVID-19 pandemic, on 30 March 2020 (see [https://en.wikipedia.org/wiki/COVID-19\\_pandemic\\_in\\_New\\_York\\_\(state\)](https://en.wikipedia.org/wiki/COVID-19_pandemic_in_New_York_(state)))). The third change-point is detected on 14 June 2020, the same day as the date when the House Appropriations Committee required the passengers to wear facial masks on public transportation. On 17 July 2020, the fourth change-point, the highest single-day increase in new confirmed cases worldwide was recorded in the US at that time. More possible explanations about detected change-points can be found in the timeline of COVID-19 in the US (2020) (see [https://en.wikipedia.org/wiki/Timeline\\_of\\_the\\_COVID-19\\_pandemic\\_in\\_the\\_United\\_States\\_\(2020\)#cite\\_note-121](https://en.wikipedia.org/wiki/Timeline_of_the_COVID-19_pandemic_in_the_United_States_(2020)#cite_note-121)).

## 8.2. *Financial Data*

We finally investigate the performance of SSAID on detecting change-points in the monthly S&P 500 close price index. These change-points can be associated with the connecting points between the bull and bear stock markets, at which the previous trend shows either a unidirectional increase or decrease, while the later trend reverses to an

opposite direction (Wecker, 1979; Frøystad and Johansen, 2017). The future price fluctuation is likely to follow the same trend after the establishment of a uni-directional trend, so it is of great importance for the investors to identify such change-points (Frøystad and Johansen, 2017). The structure of the current data is much complicated, with some obvious change-points. The amplitude jumps and their duration greatly vary in different segments, indicated by two arrows in Fig. S7 (b). As described in §4.4, our method cannot find an SNL for this kind of data set without a sliding window, thus failing to detect any change-points. The detected change-points by our method with a sliding window of 40 observations are mostly consistent with those detected by Frøystad and Johansen (2017). During the detection period, we find two longest bull markets of 61 months at two sub-periods, indicated in shaded pink areas in Fig. S7 (b) (i.e. from February 1995 to February 2000, and from January 2001 to January 2008), both of which are followed by a bear market with an obvious drop. The first longest bull market is the well-known “Dot-com Bubble”, which burst in the early 2000 (Goodnight and Green, 2010), while the second longest bull market ends at the “2007-2008 Global Financial Crisis” (McKibbin and Stoeckel, 2010).

## **9. The effect of sliding window length**

We investigate the effect of the segment length on the detection performance, by reproducing the tests shown in Fig. Fig. 9 (b), but with a range of  $L_s$ . The results are shown in Fig. S8.

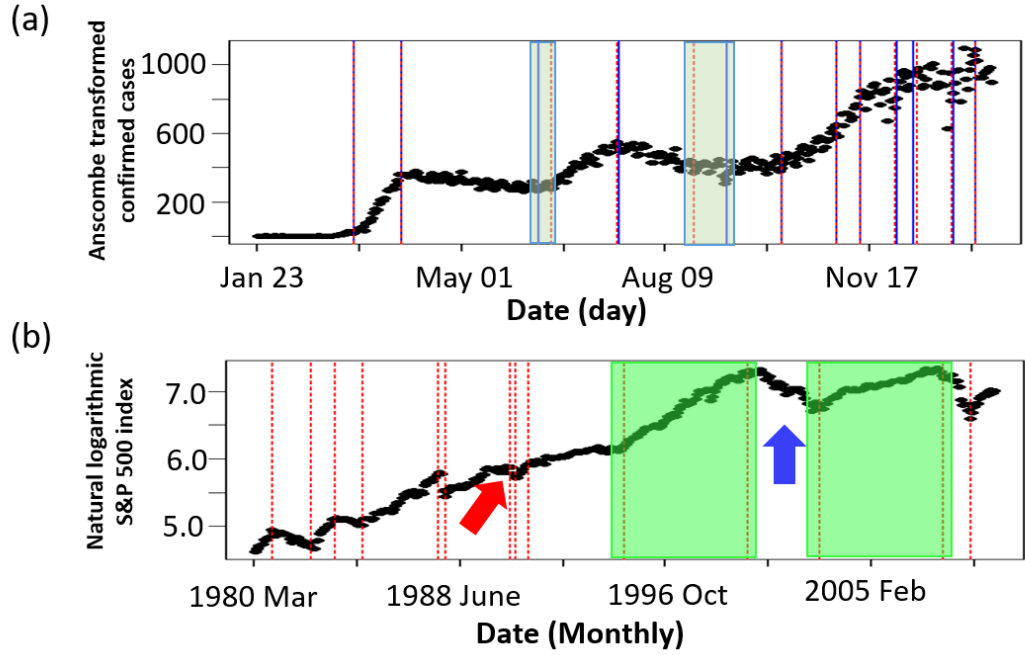

**Fig. S7.** The locations of detected change-points by SSAID in other real data sets. (a) The number of COVID-19 daily new confirmed cases in the United States. The shaded light-green areas indicate the differences of estimated change-points by different approaches in SSAID (i.e. with/without a sliding window). (b) The monthly S&P 500 close price index. The shaded green areas indicate two longest bull market identified during the period analyzed. Two arrows indicate an example showing the obvious difference in amplitude jumps between different change-points. Vertical lines: The locations of estimated change-points identified using SSAID (blue) and SSAID with sliding window (red dotted).

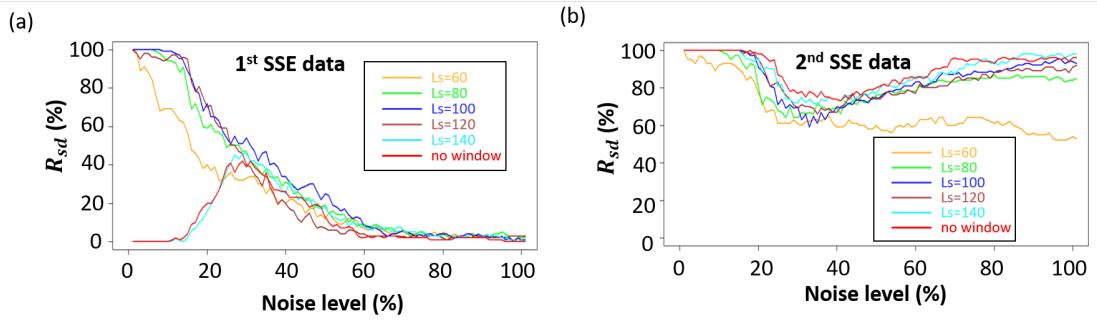

**Fig. S8.** The percentage of successful detection  $R_{sd}$  as a function of the noise level using different segment length  $L_s$  for (a) the 1<sup>st</sup> and (b) 2<sup>nd</sup> SSE data, respectively.

## References

- Anastasiou, A. and P. Fryzlewicz (2021). Detecting multiple generalized change-points by isolating single ones. *Metrika*, 1–34.
- Anscombe, F. J. (1948). The transformation of poisson, binomial and negative-binomial data. *Biometrika* 35(3/4), 246–254.
- Frøystad, A. and J. S. Johansen (2017). An analysis of bull and bear markets in the us and norway. Master’s thesis, Universitetet i Agder; University of Agder.
- Goodnight, G. T. and S. Green (2010). Rhetoric, risk, and markets: The dot-com bubble. *Quarterly Journal of Speech* 96(2), 115–140.
- Jiang, F., Z. Zhao, and X. Shao (2020). Time series analysis of covid-19 infection curve: A change-point perspective. *Journal of econometrics*.
- McKibbin, W. J. and A. Stoeckel (2010). The global financial crisis: Causes and consequences. *Asian Economic Papers* 9(1), 54–86.
- Pei, S., S. Kandula, and J. Shaman (2020). Differential effects of intervention timing on covid-19 spread in the united states. *Science advances* 6(49), eabd6370.
- Rubin, A. M. (2008). Episodic slow slip events and rate-and-state friction. *Journal of Geophysical Research: Solid Earth* 113(B11).
- Schuchat, A., C. Covid, and R. Team (2020). Public health response to the initiation and spread of pandemic covid-19 in the united states, february 24–april 21, 2020. *Morbidity and mortality weekly Report* 69(18), 551.
- Wecker, W. E. (1979). Predicting the turning points of a time series. *Journal of business*, 35–50.
